# Supplementary material for: Posterior Distillation Sampling
Source: arXiv:2311.13831 source file (2024-04-01)
Supplement: Supplementary file 1 [file supplementary.tex]

% CVPR 2024 Paper Template; see https://github.com/cvpr-org/author-kit

\documentclass[10pt,twocolumn,letterpaper]{article}

%%%%%%%%% PAPER TYPE  - PLEASE UPDATE FOR FINAL VERSION
\usepackage{cvpr}              % To produce the CAMERA-READY version
% \usepackage[review]{cvpr}      % To produce the REVIEW version
% \usepackage[pagenumbers]{cvpr} % To force page numbers, e.g. for an arXiv version

% Import additional packages in the preamble file, before hyperref
\input{header}

% It is strongly recommended to use hyperref, especially for the review version.
% hyperref with option pagebackref eases the reviewers' job.
% Please disable hyperref *only* if you encounter grave issues, 
% e.g. with the file validation for the camera-ready version.
%
% If you comment hyperref and then uncomment it, you should delete *.aux before re-running LaTeX.
% (Or just hit 'q' on the first LaTeX run, let it finish, and you should be clear).
\definecolor{cvprblue}{rgb}{0.21,0.49,0.74}
\usepackage[pagebackref,breaklinks,colorlinks,citecolor=cvprblue]{hyperref}

%%%%%%%%% PAPER ID  - PLEASE UPDATE
% \def\paperID{3012} % *** Enter the Paper ID here
 % For mula workshop

%%%%%%%%% TITLE - PLEASE UPDATE
\title{Posterior Distillation Sampling --- Supplementary Material}

%%%%%%%%% AUTHORS - PLEASE UPDATE
\author{Juil Koo $\quad$
Chanho Park $\quad$
Minhyuk Sung \\
KAIST \\
{\tt\small \{63days,charlieppark,mhsung\}@kaist.ac.kr}
}

\begin{document}
\onecolumn
\maketitle

\renewcommand{\thesection}{S}
\renewcommand{\thetable}{S\arabic{table}}
\renewcommand{\thefigure}{S\arabic{figure}}

\newif\ifpaper
\paperfalse

% \tableofcontents

% \clearpage
% \newpage

% \section*{Appendix}
\input{Sections/999_Supplementary}

{
    \small
    \bibliographystyle{ieeenat_fullname}
    \bibliography{main}
}

\end{document}
